# Supplementary material for: Towards End-to-end Unsupervised Speech Recognition
Source: arXiv:2204.02492 source file (2022-06-15)
Supplement: Supplementary file 1 [file appendix.tex]

\appendix
\onecolumn
